# Supplementary material for: Performance Analysis of UNet and Variants for Medical Image Segmentation
Source: arXiv:2309.13013 source file (2023-09-22)
Supplement: Supplementary file 1 [file appendixA.tex]

% \begin{sidewaysfigure}
  
% \end{sidewaysfigure}
