# Supplementary material for: Performance Analysis of UNet and Variants for Medical Image Segmentation
Source: arXiv:2309.13013 source file (2023-09-22)
Supplement: Supplementary file 2 [file appendixB.tex]

\section{More relevant material}
The remaining appendices can contain relevant material which is not essential to be included in the main body of the dissertation, but which may be useful to support your dissertation.

\begin{itemize}
\item	Examples of relevant material might include:
\item	Example questionnaires
\item	More detailed designs
\item	Relevant results which didn’t fit in the main body
\end{itemize}
Examples of material that should not go into an appendix:
\begin{itemize}
\item	A dump of all your code
\item	Transcripts of all your interviews
\end{itemize}
Remember, that the appendices should be there in case the reader wants to refer to them.  They will not be read as part of the dissertation story, so do not just use them to put essential material because you ran out of room.  Also, do not be tempted to pad out your dissertation to the full 60 pages just by adding lots of unnecessary material to the appendices.

Any supplementary materials can be uploaded electronically with your submission.
