# Supplementary material for: Performance Analysis of UNet and Variants for Medical Image Segmentation
Source: arXiv:2309.13013 source file (2023-09-22)
Supplement: Supplementary file 3 [file appendixC.tex]

Add your ethics letter here!!!
